# Supplementary material for: Interplay of Kondo effect and strong spin-orbit coupling in multi-hole ultraclean carbon nanotubes
Source: arXiv:1310.6530 ancillary file (2013-10-24)
Supplement: Supplementary file 1 [file SUPMAT.pdf]

# Supplemental Material for "Interplay of Kondo effect and strong spin-orbit coupling in multi-hole ultraclean carbon nanotubes"

J. P. Cleuziou, N. G. N'Guyen, S. Florens and W. Wernsdorfer
Institut Néel, CNRS et Université Joseph Fourier
BP 165, 38042 Grenoble Cedex 9
France

July 9, 2013

**Abstract**

We provide additional experimental data supporting the article. We first present complementary measurements of the device 1 discussed in the main paper, and a characterization of the relevant physical parameters. Then, we describe the device 2, showing similar features than the device 1 in the few electron regime.

## 1 Additional data of Device 1

### 1.1 Estimation of $\Delta E_{shell}$, $U$ and $\Gamma$

The mean shell spacing $\Delta E_{shell}$ is estimated from the inelastic cotunneling thresholds of the completely filled shells ($N$ = 4h). From the non-linear $dI/dV_{sd}$ conductance measurements in Fig. S1, we deduce $\Delta E_{shell} \approx 4$ meV in all shells. Besides, we also obtain the charging energy $U \approx 8$ meV, constant for the shells I-VII. Finally, the tunnel rates $\Gamma$ are estimated by a Lorentzian fit of the Coulomb peaks at finite bias (see Fig. S2) confirming the enhancement of $\Gamma$ with more negative gate voltage $V_G$ (by a roughly a factor 2 from shell VII to shell I), leading to the observed huge enhancement of $T_K$ (Fig. 3 of main text), due its the exponential behavior.

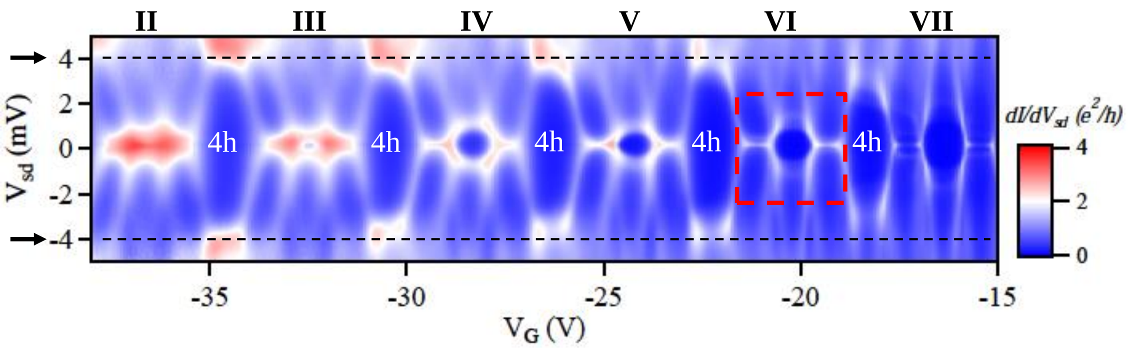


Figure S1: *Charge stability diagram of the device 1 up to larger bias voltages than in Fig. 1b of the main text. The black dashed lines indicate the inelastic cotunelling thresholds for $N = 4h$, from which we deduce $\Delta E_{shell} \approx$ 4 meV, mainly constant for the shells II-VI (except for the shell VII, where $\Delta E_{shell} \approx$ 3.3 meV).*

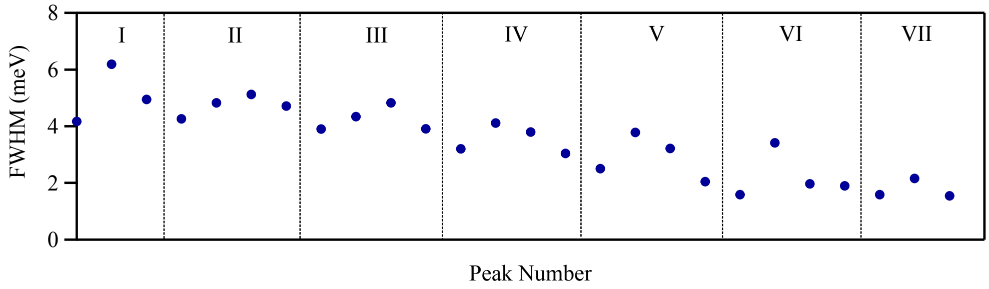


Figure S2: *Evolution of the FWHM of the Coulomb peaks associated to the successive hole fillings $N = 1h, 2h, 3h, 4h$ in shells I-VII. We used here a Lorentzian fit of the diamond edges at a fixed intermediate bias ($V_{sd}$ = -2 mV) in order to prevent the influence of the Kondo effect (at low bias) and of the next shell (at $\Delta E_{shell} \approx$ -4 mV).*

## 1.2 Cotunneling level spectroscopy under $B_{||}$-field

Here, we add some additional material concerning the spectroscopic measurements under $B_{||}$-field of the shell VI. The $d^2I/dV_{sd}^2$ plots in Fig. 2 of the main text are obtained from the numerical derivative of the measured $dI/dV_{sd}$ (see Figs. S2(b-d)), taking in the middle of the $N = 1h$, $2h$ and $3h$ valleys (along the dashed black lines in Fig. S2(a)). The orientation of the $B_{||}$-field was carefully controlled using two separate magnetic coils, thus enabling a continuous rotation of the $B$-field in the plane of the chip (see Figs. S2(e-f)).

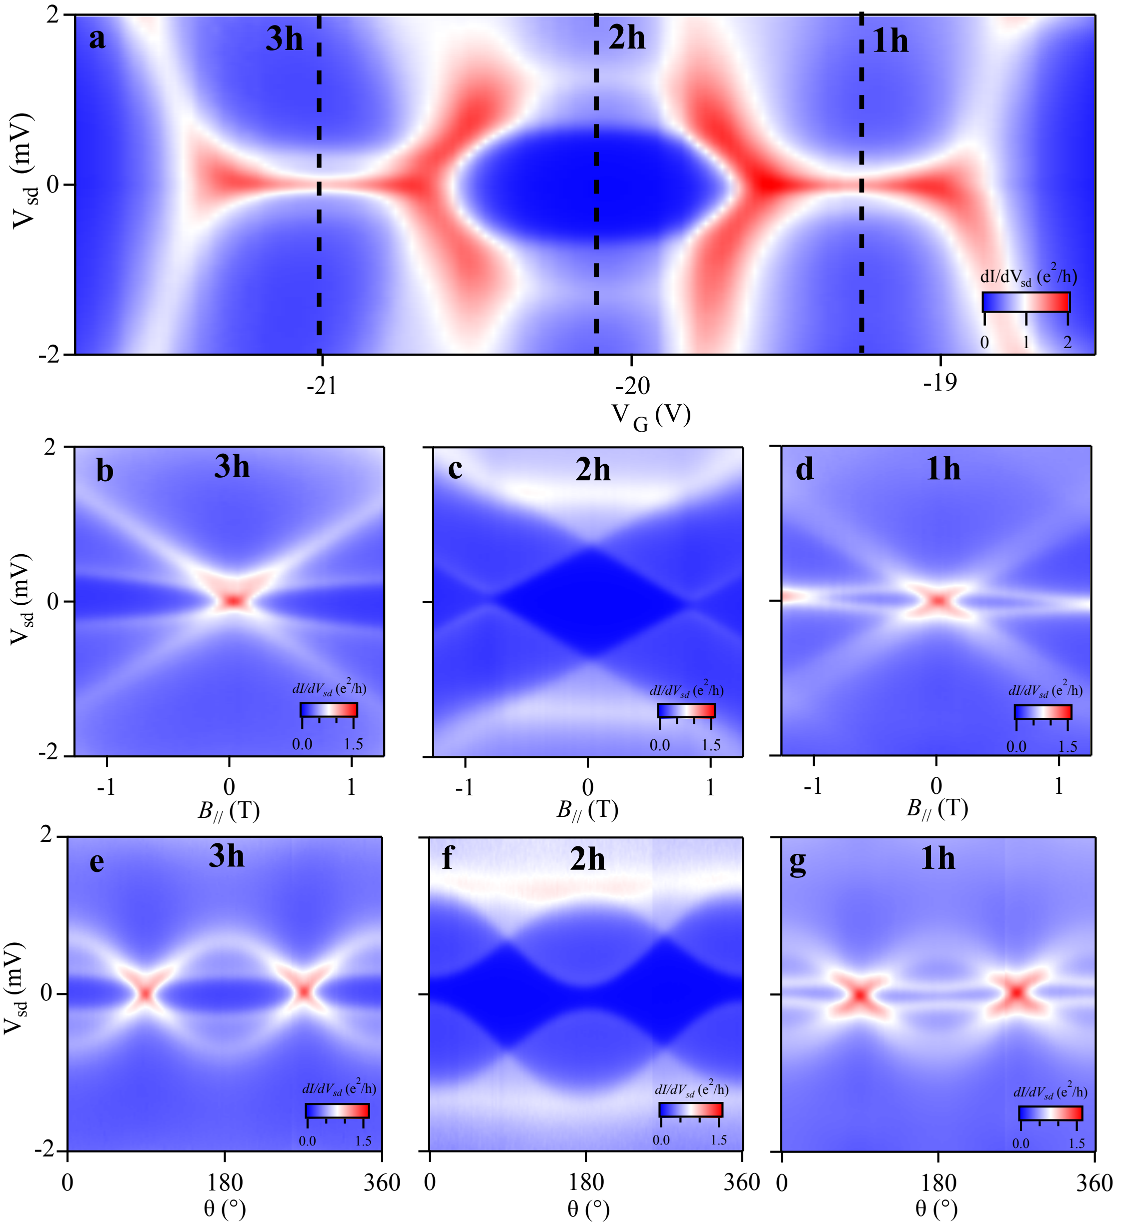


Figure S3: *Characterization of the shell VI under $B_{\|}$-field. (a) Charge stability diagram corresponding to the red dashed rectangle of Fig. S1 at $B_{\|}$ = 0. (b-d) $dI/dV_{sd}$ versus $V_{sd}$ and $B_{\|}$ measured in the $N = 3h$, $2h$ and $1h$ valleys along the black dashed line cuts in (a), respectively at $V_G$ = -21 V, -20.15 V and -19.25 V. The $d^2I/dV_{sd}^2$ colorscale plots of Fig. 2 in the main text are deduced from the numerical derivative of (d-e). (e-g) $dI/dV_{sd}$ colorscale plots, taken also in the middle of the $N = 3h$, $2h$ and $1h$ diamonds, versus $V_{sd}$ and the $B$-field angle in the sample plane ($|B|$ = 0.6 T). The orientation of the $B_{\|}$-field was determined by maximizing the orbital $g$-factor, here for $\theta$ = 0.*

## 2 Characterization of Device 2

We have measured a second ultraclean carbon nanotube device showing similar interplay of Kondo and spin-orbit physics, yet in the few electron regime. The charge stability diagram of Fig. S4 indicate here a smaller semiconducting bandgap ($E_g \approx 30$ meV) and a larger shell energy spacing ($\Delta E_{shell} \approx 8$ meV) than in device 1 . The high transparency of the tunnel barriers results here in high conductance values for the valence band (Fabry-Perot regime), while the conduction band exhibits Kondo physics already for the first few carriers (Fig. S4). The sufficiently weak tunnel coupling of the first electron shell enables to resolve the energy level spectrum under $B_{\|}$-field (Fig. S5). We obtain a very similar energy level structure than in device 1 and deduce the effective energy level splittings: $|\Delta_{SO}| \approx 0.34 \pm 0.04$ meV (note that $\Delta_{SO} < 0$), $\Delta_{VBS} \approx 0.52$ meV and $\Delta^*_{SO} \approx 1.6$ meV in the first shell. Our findings show again a strong renormalization of the effective SOI at half shell filling ($\Delta^*_{SO} \gg \Delta_{SO}$), even in the few electron regime.

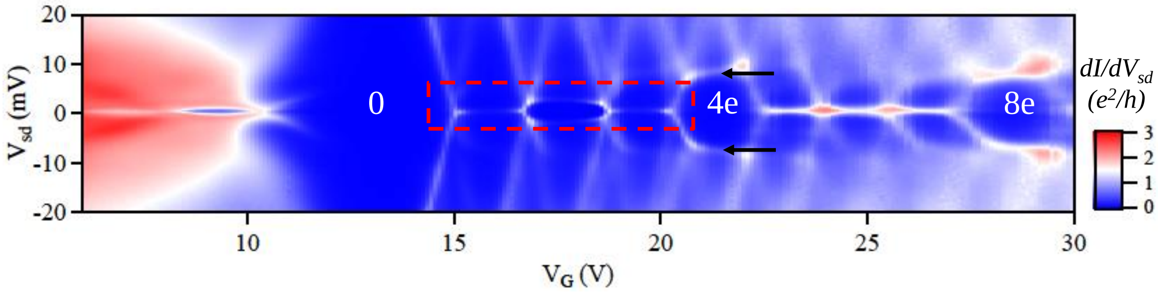


Figure S4: *Charge stability diagram of Device 2 corresponding to a small bandgap carbon nanotube ($E_g \approx 30$ meV), showing both Kondo and spin-orbit physics in the few electron regime. We estimate here a shell level spacing $\Delta E_{shell} \approx 8$ meV (see the black arrows), roughly constant for both electron shells.*

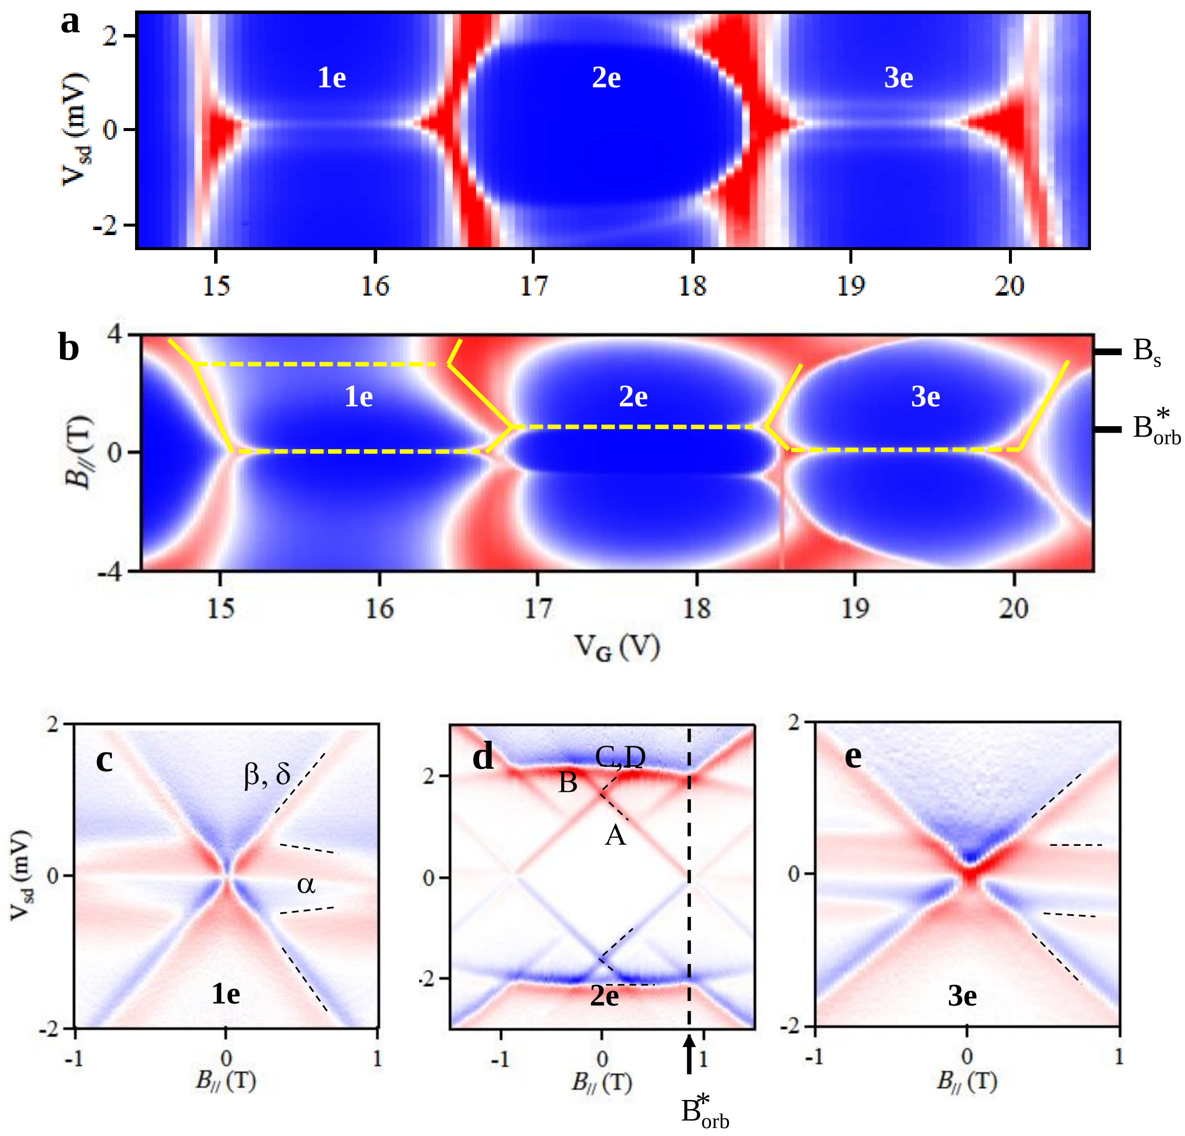


Figure S5: *Characterization of the first electron shell of Device 2 under an axial magnetic field $B_{\|}$. (a) Colorscale plot of $dI/dV_{sd}$ versus $V_{sd}$ and $V_G$ of the first electron shell at $B_{\|} = 0$ (red dashed rectangle of Fig. S4). (b) Linear differential conductance $dI/dV_{sd}$ as a function of $V_G$ showing boundaries between the first four electrons ground states under $B_{\|}$-field. The Coulomb blockade peaks (highlighted by continuous yellow lines) move with alternate upward and downward $dB_{\|}/dV_G$ slopes, resulting in kinks at the boundaries of the adjacent Coulomb blockade valleys. (c-e) $d^2I/dV_{sd}^2$ versus $B_{\|}$ and $V_{sd}$, in the middle of the $N = 1e$ (c), $2e$ (d) and $3e$ (e) diamonds, respectively. We obtain here comparable energy level spectrum than in device 1 (see Fig. 3 of main text) with a negative effective SOI sign ($\Delta_{SO} < 0$) in the conduction band and a larger orbital g-factor $g_{orb} \approx 40$ for N = 1e. The effective splittings of the energy level spectrum are: $|\Delta_{SO}| \approx 0.34 \pm 0.04$ meV for $N = 1e$, $\Delta_{VBS} \approx 0.52$ meV and $\Delta^*_{SO} \approx 1.6$ meV for $N = 2e$.*
